# Supplementary material for: Laboratory evidence of dynamo amplification of magnetic fields in a turbulent plasma
Source: arXiv:1702.03016 ancillary file (2017-02-09)
Supplement: Supplementary file 1 [file dynamo-supplementary-information.pdf]

## SUPPLEMENTARY INFORMATION

### Laboratory evidence of dynamo amplification of magnetic fields in a turbulent plasma

## Materials and Methods

### Thomson scattering

A Thomson scattering diagnostic was used to characterize various properties of the colliding jets. The Thomson scattering beam is a 30 J, 1 ns frequency doubled (526.5 nm wavelength) laser that probes the plasma within a  $50 \mu\text{m}^2$  region. The scattered light is collected with a  $63^\circ$  scattering angle and the geometry is such that the scattering wavenumber is parallel to the axis of the flow. When fitting the Thomson scattering data, a 0.025 nm instrument function was used and an electron density of  $\lesssim 10^{20} \text{ cm}^{-3}$  was assumed, as inferred from absolute calibration of the total scattered signal (see below) and predicted by FLASH simulations. Within a factor of 10 from this value for the electron density, the fitted Thomson scattering spectra showed no appreciable change. The resolution of the streak camera was  $\sim 50$  ps and so the Thomson scattering data was fitted every 100 ps.

We have investigated the potential plasma-heating effect resulting from the Thomson scattering probe beam. A simple estimate of this heating is given by [26]

$$\frac{\Delta T_e}{T_e} \lesssim 5.32 \times 10^{-7} \left( \frac{Z n_e}{T_e^{3/2}} \right) \lambda^3 (1 - e^{-\hbar\omega/eT_e}) I_0 \tau, \quad (\text{S1})$$

where  $T_e$  is the electron temperature (in eV),  $n_e$  the electron density (in  $\text{cm}^{-3}$ ),  $Z$  the mean ion charge,  $\lambda$  the laser wavelength (in cm),  $\omega$  the laser frequency,  $I_0$  the probe laser intensity (in  $\text{W}/\text{cm}^2$ ) and  $\tau$  the laser pulse duration (in s). The above equation should be regarded as an upper bound, because it does not take into account the rapid transport of heat away from the laser focus by both convection and conduction. Indeed, the high electron thermal conductivity plays an important role in making the temperature uniform in the interaction region (see below). Taking an average value of  $n_e \sim 10^{20} \text{ cm}^{-3}$  and assuming  $T_e \sim 450$  eV, we get  $\Delta T_e/T_e \lesssim 20\%$ . More quantitatively, the probe-heating effect was fully included in our FLASH simulations which predicted similar values to these simple estimates.

In order to observe the flow properties before jet collision, a single-jet experiment was carried out. The laser beams were fired on one side of the target only, and the Thomson scattering probe beam started 28 ns, after a 10 ns long laser drive. For this shot, the Thomson scattering laser beam probed the plasma on the axis of the flow, at the midpoint between the two targets.

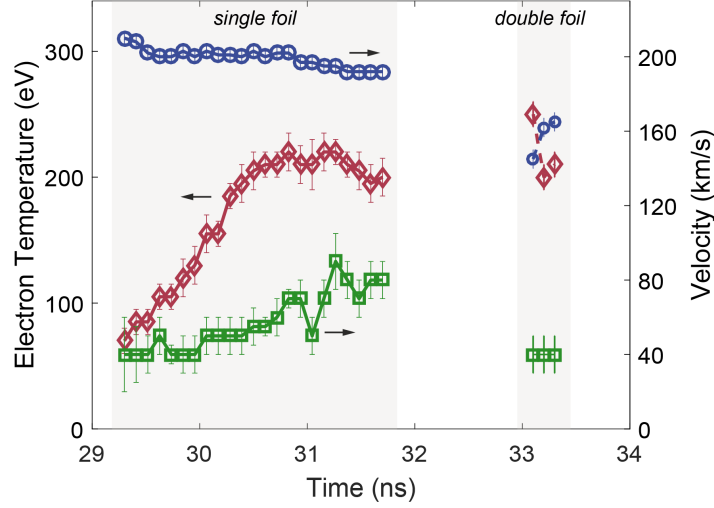

Figure 5: **Thomson scattering from a 10 ns laser drive.** Flow velocity towards grid B (full blue circles), turbulent velocity (full green squares) and electron temperature (full red diamonds) as measured by Thomson scattering for the case of a 10 ns laser drive on both a single-jet and double-jet interaction.

As shown in Figure 5, before the collision, the jets had a velocity of  $\sim 200$  km/s and electron temperature  $\sim 220$  eV.

For direct comparison with the single-jet experiment, we also used the Thomson scattering diagnostic to determine flow properties from a double-grid shot, but with a 10 ns pulse shape. In this case, the probe beam was initiated with the same timing and positioning as was used with the 5 ns laser drive (described in the main text). The results are also shown in Figure 5: the turbulent velocity for the 10 ns drive is lower than the 5 ns one, as is the associated electron temperature. Both are consistent with expected properties of the respective laser drives.

We have performed a full photometric calibration of the Thomson scattering system, recovering the electron density from each shot via a comparison between the incident and scattered power. Namely,

$$P_{scatt} = P_{inc} d\Omega r_0^2 \frac{\ell_{TS}}{2\pi} \left| \hat{s} \times \left( \hat{s} \times \hat{E}_{i0} \right) \right|^2 S(k) Z^2 n_i, \quad (S2)$$

where  $P_{scatt}$  is the scattered power,  $P_{inc}$  is the incident power of the probe beam,  $d\Omega$  is the collecting solid angle,  $r_0 = 2.818 \times 10^{-13}$  cm is the classical electron radius,  $\ell_{TS} = 50 \mu\text{m}$  is the interaction length,  $\hat{s}$  is the unit Poynting vector,  $\hat{E}_{i0}$  is the probe beam's electric field unit vector,  $S(k)$  is the spectral density function,  $Z$  is the mean ion charge and  $n_i$  is the ion density. The incident power is provided by the on-shot calorimetry performed at the Omega laser. The effective f-number of the optics was 9.1, giving a solid angle of  $10^{-2}$  sr. The spectral density

function is [26]

$$S(k) = \frac{Z\alpha^4}{(1 + \alpha^2)[1 + \alpha^2(1 + Z)]}, \quad (\text{S3})$$

which can be calculated using the previous Thomson scattering fits to the data. Here  $\alpha$  is  $1/k\lambda_D$ , with  $\lambda_D$  the Debye length. The scattered power was determined via full photometric calibration of all the optics to convert the number of detected counts (on the CCD camera) to energy. We find that for the collided jets with a 5 ns drive, the electron density was  $n_e = Zn_i \approx 7 \times 10^{19} \text{ cm}^{-3}$ , in agreement with FLASH predictions (see Figure 6).

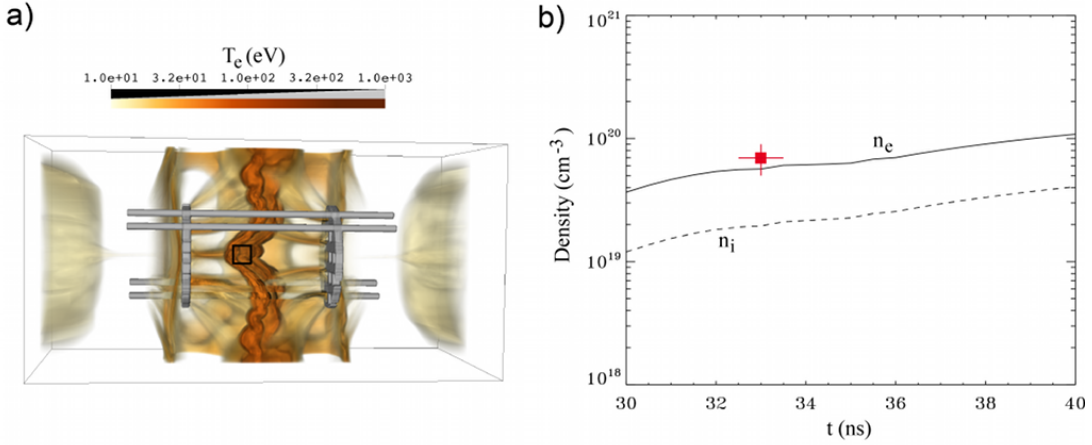

Figure 6: **FLASH temperature and density variations in the plasma.** (a) Volume rendering of  $T_e$  for the 5 ns laser drive at  $t = 35$  ns. (b) Electron density (solid line) and ion density (dashed line) profiles averaged in the jet interaction volume [the square box in panel (a)]. The red square corresponds to the estimated electron density from Thomson scattering photometric calibration.

## X-ray imaging and power spectrum of density fluctuations

The effects of turbulence on the X-ray emissivity were investigated using images of the plasma obtained from a framing camera. These images have a pixel size of  $\delta x \approx 9 \mu\text{m}$ , with an estimated resolution  $l \approx 50 - 100 \mu\text{m}$  from the pinhole size and detector sensitivity. We characterized relative fluctuations in detected intensity by performing spectral analysis of the jet-interaction region, visible approximately half-way between the grids (see Figure 2). In order to distinguish small-scale density variation from large-scale inhomogeneities of the interaction region, we constructed relative-intensity maps based on ‘coarse-grained’ mean fields calculated via a  $61 \times 61$  pixel smoothing filter – corresponding to an outer length scale  $L \approx 600 \mu\text{m}$  – combined with a two-dimensional window function to remove edge effects. Power spectra were

then calculated by taking average values from a binned annular histogram of a two-dimensional fast Fourier transform (FFT) applied to the relative-intensity image. To reduce the effect of spectral distortion due to image defects [31] such as neutron hits or striations, various filtering methods were employed. Extreme outliers were systematically detected by testing deviation from surrounding points, then removed using a median filter. Localized defects tend to appear as anisotropic features in Fourier space. Their impact on the assigned power-spectrum values was mitigated by using the median, rather than the mean, as a measure of central tendency for each bin: the former is more robust against the outlying values typically associated with such features. The efficacy of these methods was successfully tested by applying such defects on simulated Gaussian fields with prescribed spectra. To check the consistency of the spectra obtained, the above analysis was performed on multiple regions in the image, and various mean-field estimation methods were employed, including a variety of windowed regions. The jump observed in the experimental spectrum at high wavenumbers (Figure 2c) is most likely due to Poisson noise. This follows because, in the two-dimensional spectrum, Poisson noise manifests itself as a constant feature: the distortion to the predicted 1D spectrum is proportional to the wavenumber.

Fluctuations in the detected X-ray intensity are typically related to density fluctuations [32], which in turn can be related to velocity perturbations under certain conditions. The radiative energy flux (emissivity) from an optically thin plasma with  $T = T_e = T_i$  is given by a cooling function [33]

$$\epsilon = \rho \kappa_P \sigma T^4 = \kappa_0 \sigma \rho^{\alpha+1} T^{\beta+4}, \quad (\text{S4})$$

where  $\sigma$  is the Stefan-Boltzmann constant,  $\rho$  the mass density, and the functional form of the Planck opacity has been assumed to be  $\kappa_P = \kappa_0 \rho^\alpha T^\beta$ , with  $\kappa_0$  a suitable constant. For Bremsstrahlung-dominated radiation,  $\beta = -7/2$  and  $\alpha = 1$ , resulting in weak dependence on temperature [33]. Since  $\rho \propto n$ , we conclude that the emissivity can be written as

$$\epsilon = C n^{\alpha+1} T^{\beta+4}, \quad (\text{S5})$$

where  $C$  is a constant. Decomposing the number density and temperature into mean and fluctuating parts, viz.,

$$n = n_0 + \delta n, \quad T = T_0 + \delta T, \quad (\text{S6})$$

and assuming  $n_0 \gg \delta n$ ,  $T_0 \gg \delta T$ , we find that the emissivity becomes

$$\begin{aligned} \epsilon = \epsilon_0 & \left[ 1 + (\alpha + 1) \frac{\delta n}{n_0} + (\beta + 4) \frac{\delta T}{T_0} \right] \\ & + \epsilon_0 \left[ \frac{(\alpha + 1)(\alpha + 2)}{2} \frac{\delta n^2}{n_0^2} + \frac{(\beta + 4)(\beta + 5)}{2} \frac{\delta T^2}{T_0^2} \right] + \mathcal{O}\left(\frac{\delta n^3}{n_0^3}, \frac{\delta T^3}{T_0^3}\right), \end{aligned} \quad (\text{S7})$$

where the mean emissivity is  $\epsilon_0 = C n_0^{\alpha+1} T_0^{\beta+4}$ . The intensity detected on the screen is then

given by the line-of-sight integral

$$\begin{aligned}
I &= \int_0^{\ell_n} \epsilon(x, y, z) \, dz \\
&\approx I_0 + (\alpha + 1) \int_0^{\ell_n} \epsilon_0(x, y, z) \frac{\delta n}{n_0} \, dz + (\beta + 4) \int_0^{\ell_n} \epsilon_0(x, y, z) \frac{\delta T}{T_0} \, dz, \\
&+ \frac{(\alpha + 1)(\alpha + 2)}{2} \int_0^{\ell_n} \epsilon_0(x, y, z) \frac{\delta n^2}{n_0^2} \, dz + \frac{(\beta + 4)(\beta + 5)}{2} \int_0^{\ell_n} \epsilon_0(x, y, z) \frac{\delta T^2}{T_0^2} \, dz,
\end{aligned} \tag{S8}$$

with mean-field intensity  $I_0$  defined by  $I_0 \equiv \int_0^{\ell_n} \epsilon_0(x, y, z) \, dz$ , where  $\ell_n$  is the size of the plasma. Assuming  $\ell_n$  to be larger than the scale of the dominant fluctuations  $l$ , and homogeneity at small scales, we can separate the various terms with a WKB-type (Wentzel - Kramers - Brillouin) approximation to give

$$\begin{aligned}
\frac{\delta I}{I_0}(x, y) &\approx \frac{(\alpha + 1)}{\ell_n} \int_0^{\ell_n} \frac{\delta n}{n_0} \, dz + \frac{(\beta + 4)}{\ell_n} \int_0^{\ell_n} \frac{\delta T}{T_0} \, dz \\
&+ \frac{(\alpha + 1)(\alpha + 2)}{2\ell_n} \int_0^{\ell_n} \frac{\delta n^2}{n_0^2} \, dz + \frac{(\beta + 4)(\beta + 5)}{2\ell_n} \int_0^{\ell_n} \frac{\delta T^2}{T_0^2} \, dz.
\end{aligned} \tag{S9}$$

Note that we cannot necessarily neglect the quadratic terms in (S9), because the linear integrals are reduced in magnitude by a factor  $(l/\ell_n)^{1/2}$  due to the fluctuating integrands; this reduction is not seen in the quadratic terms. In order to ignore the latter, we would require  $\delta n/n_0 < (l/\ell_n)^{1/2}$  and  $\delta T/T_0 < (l/\ell_n)^{1/2}$ . Yet, for 1D power spectra shallower than  $k^{-2}$  this condition is not satisfied.

To proceed further, we need to use an equation of state to relate density and temperature fluctuations. For example, in the case of subsonic, ideal gas motions, it can be shown from pressure balance that

$$\frac{\delta n}{n_0} \approx -\frac{\delta T}{T_0}. \tag{S10}$$

This gives a quadratic relation between intensity and density fluctuations of the form

$$\frac{\delta I}{I_0}(x, y) \approx \frac{c_1}{\ell_n} \int_0^{\ell_n} \frac{\delta n}{n_0}(x, y, z) \, dz + \frac{c_2}{\ell_n} \int_0^{\ell_n} \frac{\delta n^2}{n_0^2}(x, y, z) \, dz, \tag{S11}$$

provided  $c_1$  and  $c_2$  do not vanish. Alternatively, a similar result can be obtained by assuming that the temperature remains uniform in the plasma, thus neglecting temperature fluctuations with respect to density fluctuations. Since thermal conductivity is large in our experiment, such an assumption would be reasonable; furthermore, a relatively uniform temperature across the interaction region is predicted by FLASH simulations (see Figure 6a). The above considerations allow the (assumed homogeneous) intensity and density correlation functions, defined by

$$C^{(I)}(\mathbf{x}'_{\perp} - \mathbf{x}_{\perp}) = \left\langle \frac{\delta I}{I_0}(\mathbf{x}_{\perp}) \frac{\delta I}{I_0}(\mathbf{x}'_{\perp}) \right\rangle, \tag{S12}$$

$$C^{(n)}(\mathbf{x}' - \mathbf{x}) = \left\langle \frac{\delta n}{n_0}(\mathbf{x}) \frac{\delta n}{n_0}(\mathbf{x}') \right\rangle, \quad (\text{S13})$$

$$C^{(n^2)}(\mathbf{x}' - \mathbf{x}) = \left\langle \frac{\delta n^2}{n_0^2}(\mathbf{x}) \frac{\delta n^2}{n_0^2}(\mathbf{x}') \right\rangle, \quad (\text{S14})$$

to be related via

$$C^{(I)}(\mathbf{x}'_{\perp} - \mathbf{x}_{\perp}) = \frac{c_1^2}{\ell_n} \int_{-\infty}^{\infty} C^{(n)}(\mathbf{x}'_{\perp} - \mathbf{x}_{\perp}, r_z) dr_z + \frac{c_2^2}{\ell_n} \int_{-\infty}^{\infty} C^{(n^2)}(\mathbf{x}'_{\perp} - \mathbf{x}_{\perp}, r_z) dr_z, \quad (\text{S15})$$

where we have used typical decay conditions on the density correlation function to extend the integrals formally over the entire real line, and have neglected the cross-correlation between  $\delta n/n_0$  and  $\delta n^2/n_0^2$  on the grounds that such a term contains the same reduction factor as the linear term, and so is negligible under the small fluctuation assumption  $\delta n/n_0 \ll 1$ .

The 2D intensity spectrum  $P_{2D}(\mathbf{k}_{\perp})$ , 3D density spectrum  $P_{3D}(\mathbf{k})$ , and 3D squared-density spectrum  $P_{3D}^{(2)}(\mathbf{k})$ , given by the Fourier transforms of (S12), (S13), and (S14), respectively, combined with the Wiener-Khinchin Theorem [34], are therefore related by

$$P_{2D}(\mathbf{k}_{\perp}) = \frac{c_1^2}{\ell_n} P_{3D}(\mathbf{k}_{\perp}, 0) + \frac{c_2^2}{\ell_n} P_{3D}^{(2)}(\mathbf{k}_{\perp}, 0) = \frac{c_1^2}{\ell_n} P_{3D}(k_{\perp}) + \frac{c_2^2}{\ell_n} P_{3D}^{(2)}(k_{\perp}). \quad (\text{S16})$$

Isotropy of the statistics of the power spectrum was invoked for the last equality. We simplify (S16) by noting that  $P_{3D}^{(2)}(k)$  can be written

$$P_{3D}^{(2)}(k) \equiv \left\langle \left| \left( \frac{\delta n^2}{n_0^2} \right)_{\mathbf{k}} \right|^2 \right\rangle = \left\langle \frac{1}{n_0^4} \left| \sum_{\mathbf{k}'} \delta n_{\mathbf{k}'} \delta n_{\mathbf{k}-\mathbf{k}'} \right|^2 \right\rangle = \frac{1}{n_0^4} \sum_{\mathbf{k}', \mathbf{k}''} \langle \delta n_{\mathbf{k}'} \delta n_{\mathbf{k}-\mathbf{k}'} \delta n_{\mathbf{k}''}^* \delta n_{\mathbf{k}-\mathbf{k}''}^* \rangle. \quad (\text{S17})$$

On account of the largest density fluctuations occurring at the smallest wavenumbers, the sum is dominated by wavemodes where  $k', k'' \ll k$ , so (S17) becomes

$$P_{3D}^{(2)}(k) \approx \frac{1}{n_0^4} \sum_{\mathbf{k}', \mathbf{k}''} \langle \delta n_{\mathbf{k}'} \delta n_{\mathbf{k}} \delta n_{\mathbf{k}''}^* \delta n_{\mathbf{k}}^* \rangle \approx \left\langle \left| \frac{\delta n_{\mathbf{k}}}{n_0} \right|^2 \right\rangle \sum_{\mathbf{k}', \mathbf{k}''} \left\langle \frac{\delta n_{\mathbf{k}'}}{n_0} \frac{\delta n_{\mathbf{k}''}^*}{n_0} \right\rangle = P_{3D}(k) \left\langle \frac{\delta n^2}{n_0^2} \right\rangle. \quad (\text{S18})$$

The validity of this last step can be tested with artificial fields, and numerical results do indeed support it. The desired relation

$$P_{3D}(k) \propto P_{2D}(k) \quad (\text{S19})$$

follows from (S18) applied to (S16).

In the subsonic regime, this relationship should hold more generally than for an ideal gas, provided any linearized relationship deduced between density and temperature fluctuations from the equation of state does not lead to the coefficients  $c_1$  and  $c_2$  vanishing in the quadratic-intensity result (S11).

## Faraday rotation

We have implemented Faraday rotation measurements in the plasma using the Thomson scattering diagnostic system already available at the Omega laser facility. Using a Wollaston prism, the Thomson scattered light beam was separated into two orthogonal components,  $S$  and  $P$ . The magnitude of the detected  $S$  and  $P$  polarizations  $I_S$  and  $I_P$  depends on three factors: the initial polarization of the linearly-polarized probe beam, the relative transmission of the  $S$  and  $P$  components through the diagnostic optics subsequent to their separation by the prism, and changes to polarization due to Faraday rotation. Namely,

$$I_S = A_S I_0 \sin^2 (\theta_c + \Delta\theta), \quad (\text{S20})$$

$$I_P = A_P I_0 \cos^2 (\theta_c + \Delta\theta), \quad (\text{S21})$$

where  $I_0$  is the probe laser intensity,  $A_S$  and  $A_P$  the (distinct) transmission factors for each polarization,  $\theta_c$  the angle at which the  $S$  and  $P$  components are split by the prism, and  $\Delta\theta$  the rotation due to the Faraday effect. Taking the ratio of (S20) and (S21), we find

$$\tan^2 (\theta_c + \Delta\theta) = \frac{A_P}{A_S} \frac{I_S}{I_P}. \quad (\text{S22})$$

If  $\theta_c$  and the ratio  $A_S/A_P$  are known, the degree of Faraday rotation  $\Delta\theta$  can be calculated from  $I_S/I_P$ .

In this experiment, the Faraday rotation diagnostic was set up so that the  $S$  and  $P$  components are equally split by the prism, that is  $\theta_c = 45^\circ$ . To calculate the transmission ratio, we consider the magnitude of the two components for a single jet case. The single-jet case can be used for calibration, because the proton radiography diagnostic indicates that the magnetic fields are small enough that the Faraday rotation angle is below detector sensitivity. In Figure 7, we show the raw image of the split polarizations and plot the summed intensity of the signal for its entire duration. We determine the transmission ratio to be  $A_S/A_P = 0.43$ . The use of this data for calibration is validated by the fact that the measured rotation angle remains constant in time, as shown in Figure 3c in the main text. Since the resolution of the streak camera is  $\sim 50$  ps, the Faraday rotation angle for other shots is then calculated at 100 ps intervals.

When the Faraday-rotation angle is small, it is given (in Gaussian units) by [34]

$$\Delta\theta = \frac{\lambda^2 e^3}{2\pi m_e^2 c^4} \int_0^{2\ell_n} n_e(s) B_{\parallel}(s) ds. \quad (\text{S23})$$

It is appropriate to use twice the size of the plasma  $\ell_n$  for the path length of the integral because the geometry of the jet-interaction region is such that the Thomson scattering volume lies on the opposing side to that from which the probe beam originates. The incident laser's wavelength is  $\lambda = 5.27 \times 10^{-5}$  cm, so this implies

$$\int_0^{2\ell_n} n_e(s) B_{\parallel}(s) ds = 2.4 \times 10^{23} \Delta\theta \text{ G cm}^{-2}. \quad (\text{S24})$$

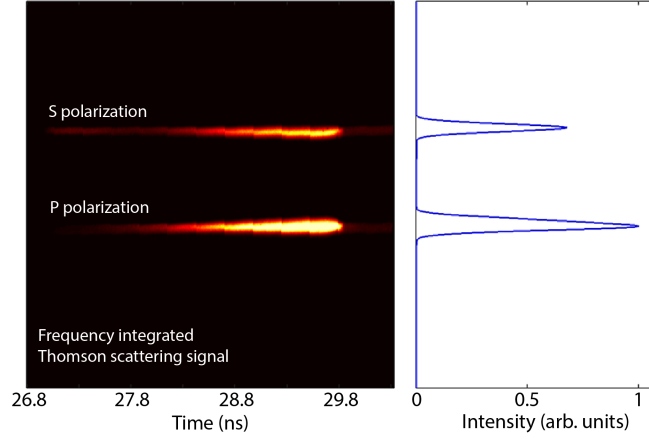

Figure 7: **Faraday-rotation calibration.** Total Faraday-rotation signal for the two polarizations for the case of a single jet driven with a 10 ns pulse profile.

If the mean magnetic field is small or zero, the mean of the Faraday-rotation measure should vanish and so measured values of it correspond to the standard deviation of the line-of-sight integral in (S24). This can be estimated by a random-walk argument: assuming a random field has correlation scale  $\ell_B$ , the typical deviation is equal to the deviation acquired across one correlated structure multiplied by the square root of the number of such structures encountered. (S24) then implies

$$\sqrt{\ell_n \ell_B} n_e B_{\parallel} \sim 1.7 \times 10^{23} \Delta\theta \text{ G cm}^{-2}, \quad (\text{S25})$$

where  $\ell_n$  is the length scale of the density profile and  $\ell_B$  the scale of the magnetic structures that have the largest amplitude. This estimate can be re-arranged to give the result stated in the main text.

There are a range of effects to which the probe beam is subject but that can be reasonably neglected in our analysis. The probe laser changes frequency – and hence wavelength – after scattering, due to collective plasma effects in the probe-interaction region; however, the largest such change will be of the order of the plasma frequency, and this corresponds to a maximum wavelength shift  $\Delta\lambda/\lambda \lesssim 30\%$ . The error in Faraday rotation associated to this wavelength modification is  $\lesssim 20\%$ , which is less than the noise in the streak camera data. Due to the small size of the electron Larmor frequency ( $\Omega_e \approx 2 \times 10^{12} \text{ s}^{-1}$ ) compared to the laser frequency ( $\omega \approx 4 \times 10^{15} \text{ s}^{-1}$ ), it can also be shown that other magnetic effects on the polarization – such as the Cotton-Mouton effect – are much smaller in magnitude than the experimental error [36] and can be safely omitted.

## Proton radiography

Proton deflections in the proton radiography diagnostic are primarily due to magnetic fields rather than electric fields or effects such as Coulomb collisions and kinetic beam instabilities. This can be seen from the energy map on the CR-39 plates. Figure 8 shows that, in the jet-interaction region, the mean proton energy has a uniform distribution without pronounced density structures.

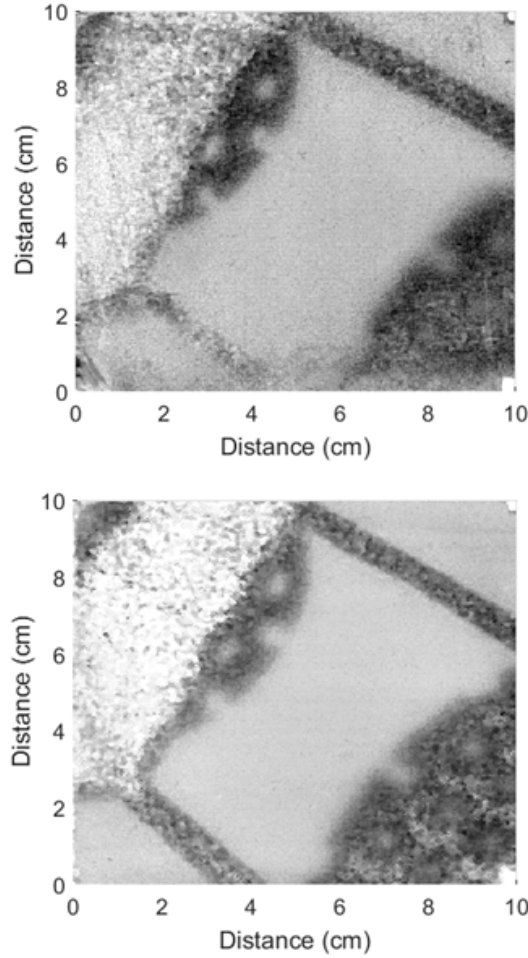

Figure 8: **Mean proton energy.** Mean proton energy vs. position for the 15.0 MeV protons recorded on the CR-39 plate. The distribution is very uniform, indicating that the structures seen in the flux images (see Figures 4c and 4d in the main text) are due to deflections of protons by magnetic fields. Top: Target with both grids, and with the two chlorinated plastic foils driven with a 10 ns long pulse shape. The  $D^3He$  capsule was imploded at  $t = 34$  ns. Bottom: same as above but with a 5 ns laser driver

For arbitrary magnetic-field configurations and imaging beam parameters, relating analytical distributions of flux and the magnetic fields from which they arise is non-trivial. However, for radiographic set-ups similar to (and including) this experiment, a number of simplifications can be made to improve tractability of the “reconstruction” problem of extracting path-integrated magnetic fields directly from a given proton flux distribution. Based on such an approach, here we discuss the formulae used to derive the images of path-integrated fields, shown in Figure 4 of the main text, as well as the assumptions under which these formulas are valid. A full derivation of these results is presented elsewhere [37].

We calculate path-integrated fields from the experimentally obtained proton-flux images, assuming that the distribution of flux  $\Psi$  is related to the path-integrated field by a Monge-Ampère equation [38] of the form

$$\Psi(\nabla\phi(\mathbf{x}_{\perp 0})) = \frac{\Psi_0}{|\det \nabla\nabla\phi(\mathbf{x}_{\perp 0})|} . \quad (\text{S26})$$

In this expression,  $\nabla \equiv \partial/\partial\mathbf{x}_{\perp 0}$  is a gradient operator defined on a two-dimensional coordinate system  $\mathbf{x}_{\perp 0}$  co-planar with the imaging screen (CR-39 plate), but with a scale reduced by the imaging magnification factor

$$\mathcal{M} \approx \frac{r_s + r_i}{r_i} \approx 28 , \quad (\text{S27})$$

where  $r_s \approx 27$  cm is the distance from the plasma to the screen and  $r_i \approx 1$  cm is the distance from the proton source to the plasma.  $\Psi_0$  is the initial uniform flux distribution, but with its magnitude multiplied by a scaling factor of  $\mathcal{M}^{-2}$ .  $\nabla\phi$  is a two-dimensional gradient map related to the path-integrated magnetic field by

$$\nabla\phi(\mathbf{x}_{\perp 0}) = \mathbf{x}_{\perp 0} + \frac{r_s r_i}{r_s + r_i} \frac{e}{m_p c v_p} \hat{\mathbf{z}} \times \int_0^{l_i} ds \mathbf{B}[\mathbf{x}(s)] , \quad (\text{S28})$$

where  $e$  is the proton charge,  $m_p$  the proton mass,  $v_p$  the proton speed,  $\hat{\mathbf{z}}$  a unit vector perpendicular to the imaging screen,  $l_i$  the size of the plasma,  $s$  the path length, and  $\mathbf{x}(s)$  the trajectory of a proton through the plasma with initial position  $\mathbf{x}_0 = (\mathbf{x}_{\perp 0}, 0)$  and velocity  $\mathbf{v}_0$ . The gradient map defined by (S28) does not include explicitly the imaging magnification factor  $\mathcal{M}$ , which is instead incorporated into the scheme via the re-scaled initial flux  $\Psi_0$ . Although (S26) is non-linear, it has a unique solution for  $\nabla\phi$  given any (positive) flux distribution  $\Psi$  with a boundary condition

$$\hat{\mathbf{n}} \cdot \nabla\phi(\mathbf{x}_{\perp 0}) = \hat{\mathbf{n}} \cdot \mathbf{x}_{\perp 0} \quad \text{on } \delta S, \quad (\text{S29})$$

where  $\delta S$  is the boundary of the region containing the flux distribution of interest, and  $\hat{\mathbf{n}}$  the normal to that boundary [38].

The flux relation (S26) with boundary condition (S29) was inverted numerically using a finite-difference scheme applied to the parabolic Monge-Ampère equation, the steady-state solution of which is the solution of the conventional Monge-Ampère equation [39]. In implementing this field-reconstruction algorithm for actual data, two filtering procedures were utilized.

First, a Lucy-Richardson deconvolution algorithm was applied to flux images [40, 41]. This is because the strength of path-integrated fields predicted by solving the Monge-Ampère equation is reduced in the case where strong, narrow flux features are affected by finite image resolution (“smearing”). Some of these effects, such as stochastic magnetic diffusion due to small-scale fields, are difficult to eliminate, due to unknown parameters associated with smearing. However, the effect on image resolution due to the finite size of the proton source has been shown to be a convolution of the “unsmeared” flux image resulting from a point proton source with a point-spread function whose precise form is determined by the velocity profile of the protons [37]. In the case of a fusion capsule, this point-spread function has been well-described as Gaussian, with full-width-half-maximum (FWHM) of  $50\mathcal{M} \mu\text{m} \approx 0.14 \text{ cm}$  when including the imaging-magnification factor [42, 43]. Assuming such a point-spread function for the experimental data, the Lucy-Richardson deconvolution scheme was then implemented. For the particular flux images shown in Figures 4 and 9, ten iterations were found to balance optimally the recovery of the flux distribution with the undesired side effect of Poisson noise enhancement introduced by the deconvolution process. The efficacy of the deconvolution scheme is further enhanced by the general robustness of the non-linear reconstruction algorithm to small-scale noise [37]. An illustration of successful application of Lucy-Richardson deconvolution for simulated FLASH proton radiography is given later (Figure 11).

In addition to the deconvolution, a Gaussian high-pass filter (FWHM  $2.2\mathcal{M}l_i \approx 6.16 \text{ cm}$ ) was applied to a selected flux region, in order to remove long-scale variation in the flux distribution. This procedure is required because, when implemented practically, the initial flux produced by fusion capsules can vary by as much as 50% across a single CR-39 sample, though variations over solid angles  $\leq 1.1^\circ$  are typically small compared to the mean flux [44]. Since the dominant structures remaining in the reconstruction are of the order  $l_B \sim 300 \mu\text{m}$ , and order-unity flux features are still retained in the filtered flux image, we conclude that our field-reconstruction algorithm captures the energetically dominant magnetic structures.

The flux regions of interest (shown in Figure 4 between the grids and rods) typically have irregular shapes; to make them compatible with a rectangular finite-difference grid, we embed each section of flux in a larger rectangular region, with the edge filled with uniform mean flux (as calculated from the chosen sample). The initial flux is then chosen to be entirely uniform, with mean value set equal to that of the experimental flux region. The reconstruction algorithm is then applied, with (S29) specified on the boundary of the larger rectangular region. With the reconstruction completed, an image of the magnitude of the calculated path-integrated field is then re-oriented to the original position of its associated flux region.

The applicability of this scheme to our radiography set-up depends on various assumptions: paraxiality, small deflections, point-projection, and radiographic injectivity. Since the distance  $r_i$  from the proton source to the plasma is much greater than the size  $\ell_n$  of the plasma, we can approximate the section of the beam passing through the plasma as planar, despite the fact that proton beams generated by fusion reactions in a  $\text{D}_2$  capsule implosion generally take the form of a uniformly expanding spherical shell [43]. For a given proton, this paraxial approximation is effectively an expansion of the position and velocity of the particle in terms of the paraxial

parameter

$$\varphi_0 \equiv \frac{\ell_n}{2r_i} \ll 1, \quad (\text{S30})$$

the ratio of the size  $\ell_n$  of the region being imaged to the radius  $r_i$  of curvature. For our experiment, we have  $\ell_n \approx 0.06$  cm,  $r_i \approx 1$  cm, giving  $\varphi_0 \approx 0.03 \ll 1$ , as required. This means that the initial velocity  $\mathbf{v}_0$  of a proton with initial position  $\mathbf{x}_0$  before interaction with magnetic fields can be written as

$$\mathbf{v}_0 = v_p \left( \hat{\mathbf{z}} + \frac{\mathbf{x}_{\perp 0}}{r_i} \right). \quad (\text{S31})$$

Next, typical proton-velocity deflections are assumed small compared to the initial proton velocity. More precisely, it can be shown by integrating the equations of motion under this assumption that a proton with initial position  $\mathbf{x}_0$  and velocity  $\mathbf{v}_0$  acquires a velocity perturbation  $\mathbf{w}$  due to magnetic forces given by

$$\mathbf{w} \approx \frac{e}{m_p c v_p} \mathbf{v}_0 \times \int_0^{l_i} ds \mathbf{B}(\mathbf{x}(s)) \approx \frac{e}{mc} \hat{\mathbf{z}} \times \int_0^{l_i} ds \mathbf{B}(\mathbf{x}(s)). \quad (\text{S32})$$

The second approximation is obtained by substituting the initial velocity (S31) and neglecting  $\mathcal{O}(\varphi_0)$  terms. Equation (S32) implies that the deflection velocity of a proton is perpendicular to its initial direction – that is,  $\mathbf{w} \cdot \mathbf{v}_0 \approx \mathbf{w} \cdot \hat{\mathbf{z}} \approx 0$  – and so the deflection angle of the proton is given by

$$\Delta\varphi \equiv \frac{|\mathbf{w}|}{v_p} \sim \frac{eB\ell_n}{mcv_p}. \quad (\text{S33})$$

For our experiment, Figure 4f shows that the maximum predicted path-integrated magnetic field takes a value of 6 kG cm, which in turn gives maximum predicted deflection velocity  $w \approx 5.7 \times 10^7$  cm/s. For the slowest species of proton used for imaging (3.3 MeV), we have  $v_p \approx 2.5 \times 10^9$  cm/s, so  $\Delta\varphi \leq 0.02$  for all imaging protons. For magnetic fields varying over shorter length scales, this value is further reduced.

The point-projection assumption – that the distance  $r_s$  from the plasma to the screen is much greater than  $\ell_n$  – also holds, meaning that displacements from undeflected proton trajectories acquired inside the plasma due to magnetic forces are negligible compared to the displacements resulting from the free motion of particles after they have exited the plasma, with deflected velocity.

The mapping equation (S26) implicitly assumes that no trajectories cross before the protons reach the screen, i.e., that the gradient map (S28) is injective. It is not necessarily clear from any particular image whether or not it is injective, an issue discussed at length in [37]. Non-injective images can occur in radiographic set-ups, and are typically characterized by strong flux features known as caustics, which can be hard to distinguish from strong yet injective flux structures in the presence of effects limiting spatial resolution (smearing effects), such as finite proton-source size. Applying a field-reconstruction algorithm to an image formed by a non-injective gradient map can lead to inaccurately inferred magnetic field morphologies, and

underestimates of field strengths [37]. Indeed, the solution of the Monge-Ampère equation is known to provide a lower bound on the RMS of all path-integrated field strengths that can generate a particular flux distribution [38]. However, we claim that for the 15.0 MeV proton images from our experiment, non-injectivity of the gradient map would not significantly alter the reconstructed path-integrated field. The justification of this claim is given in subsequent paragraphs.

An alternative test of the field reconstruction algorithm can be carried out by generating an artificial proton flux image, with the deflections of simulated protons determined by the reconstructed path-integrated field combined with (S32) (see Figure 9a). The test consists in comparing these synthetic images to the experimental ones. The result is that they agree fairly well, although the strength of the strong, narrow flux features in the predicted flux image is reduced compared to the experimental one. Enhancing the path-integrated field by 20% recovers the observed strength of flux features (see Figure 9b), suggesting that the reconstructed path-integrated field as shown in Figure 4f is marginally underestimated.

The imploding capsule also produces 3.3 MeV protons from DD reactions, with associated smaller velocity  $v \approx 2.5 \times 10^9$  cm/s. These slower protons are recorded independently from the faster, 15.0 MeV protons; the DD equivalents of the  $D^3He$  images (displayed in Figure 4 of the main text) are shown in Figure 10. Similar order-unity flux structures can be seen in these 3.3 MeV proton images, as expected from the inverse velocity dependence of the small-deflection angle criterion (S33). The similar positioning of these flux structures to structures present in 15.0 MeV proton images is intuitively less obvious, but matches previous findings both for simple analytic cases and other experiments [45]. The increased thickness of the structures in Figure 9 compared to those in the 15.0 MeV flux images is consistent with the existence of caustics in the former. As a result, applying the field-reconstruction algorithm to the 3.3 MeV images gives path-integrated fields that underestimate field strength compared to those recovered from the 15.0 MeV images.

Despite the presence of caustics, the 3.3 MeV proton radiographs can be used to verify the assumption of injectivity of the 15.0 MeV images. The turnover time of the plasma motions ( $L/u_L \sim 6$  ns) is much greater than the difference in transit time of the two species of protons used for imaging ( $\leq 0.2$  ns). Therefore, to a good approximation, the 3.3 MeV and 15.0 MeV protons are deflected by the same magnetic fields. As a result, any path-integrated field reconstructed from the flux image of one proton species should be consistent with flux images obtained for the other species. This can be tested by generating a predicted image using a reconstructed field from one proton species combined with mapping (S28), but varying the initial proton speed to match that of the other proton species. When such a test is carried out for the 15.0 MeV proton reconstructions, the morphology of predicted 3.3 MeV proton images agrees well with the actual 3.3 MeV proton images – see Figure 9c for example. Further, numerical experiments investigating the use of our reconstruction algorithm in the regime where caustic appearance cannot be detected by the test given above suggest that the predicted path-integrated field morphology remains relatively robust, though field strength can be somewhat underestimated [37]. This is consistent with the observation (see Figures 9b and 9d) that a 20% increase

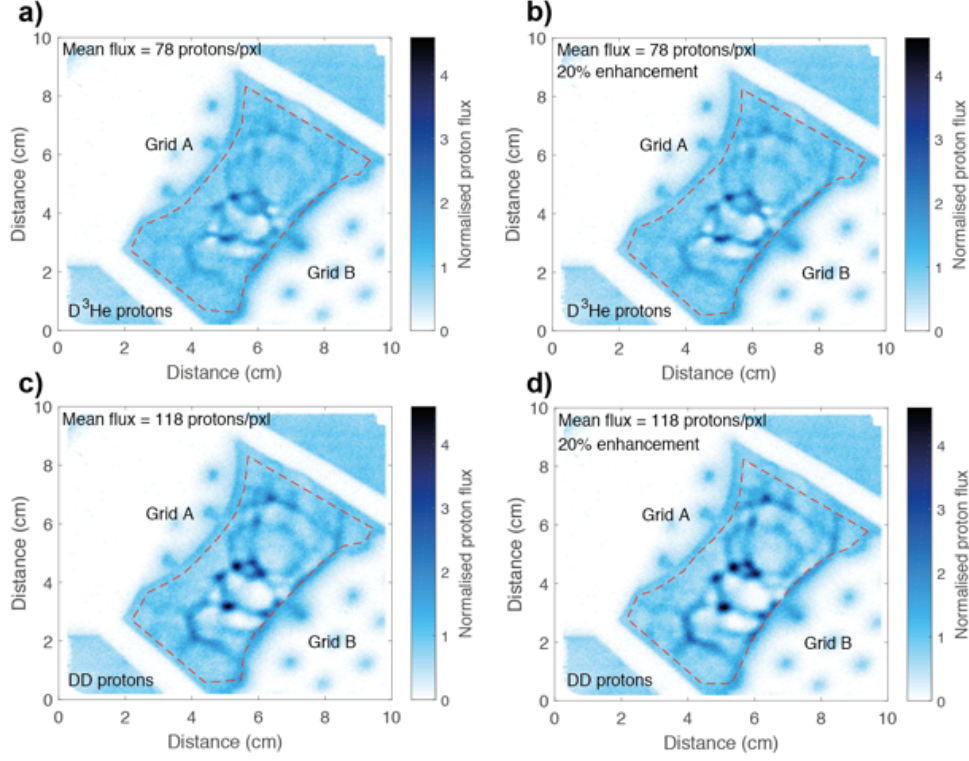

**Figure 9: Validation of field reconstruction algorithm.** (a) 15.0-MeV flux image predicted using reconstructed path-integrated magnetic field shown in Figure 4f (cf. Figure 4c). The image is created by seeding uniformly test protons in the region over which the path-integrated field is defined (marked by a dashed red line), before assigning velocities to those particles. These velocities are given by the combination of a particle's initial velocity (S31) before interacting with fields, and velocity perturbation (S32) due to magnetic fields. The particles are then allowed to propagate to the screen, with dimensions set equal to those in the experiment. The mean flux in each region is set equal to the mean flux of the experimental image. To account for finite source size, a Gaussian point spread function with FWHM  $50 \text{ } \mu\text{m} \approx 0.14 \text{ cm}$  is subsequently applied to the images. (b) Same as (a), but with the strength of the path-integrated field increased by 20%. (c) 3.3-MeV flux image predicted using reconstructed path-integrated magnetic field shown in Figure 4f (cf. Figure 10d). The path-integrated field experienced by the slower proton species is the same, but their initial perpendicular velocity is reduced, leading to larger deflections. (d) Same as (a), but with the strength of the path-integrated field increased by 20%.

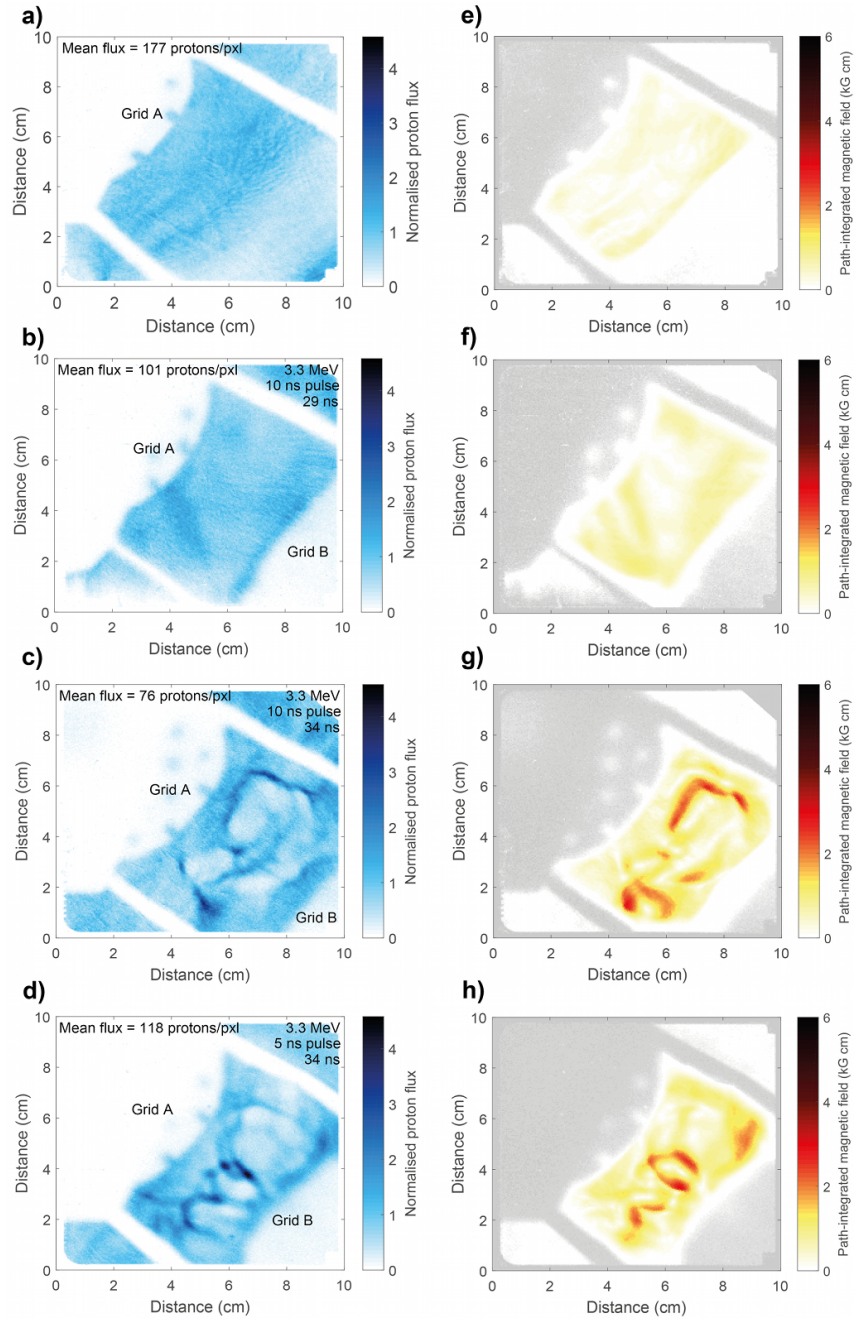

Figure 10: **Lower-energy proton radiography.** Radiographs displaying DD 3.3 MeV proton flux as recorded on the CR-39 plate. (a) Capsule implosion at  $t = 22$  ns, with only one foil, driven using a 10 ns laser pulse. (b) Capsule implosion at  $t = 29$  ns, with both foils, driven with a 10 ns laser pulse. (c) Same as (b) but at  $t = 34$  ns. (d) Same as (c) but driven with a 5 ns pulse.

in field strength still leads to similar flux features.

The spectrum of magnetic field energy  $E_B(k)$  can be calculated directly from the path-integrated magnetic field if the field's statistics are assumed isotropic [37]. Specifically, the experimental spectra shown in Figure 2 and Figure 11 are calculated using

$$E_B(k) = \frac{1}{4\pi^2\ell_n} k E_{path}(k) , \quad (\text{S34})$$

where  $E_{path}(k)$  is the one-dimensional spectrum of the path-integrated magnetic field. The RMS value of the magnetic field can then be evaluated by integrating over all wavenumbers to give

$$B_{rms}^2 = 8\pi \int_0^\infty E_B(k) dk . \quad (\text{S35})$$

In practice, the values of the RMS field strength given in the main paper are calculated by summing over pixel values of a Fourier-transformed sample of zero-mean path-integrated magnetic field (the region denoted by a dashed curve in Figure 4f). Prior to the jet collision, the electron-density scale length is larger, of order the grid's lateral dimensions  $\ell_n \geq 3$  mm (we know this from FLASH simulations). However, as the collision occurs, and the turbulent jet-interaction region forms, the density scale increases to  $\ell_n \sim 0.6$  mm, as stated in the main text.

We have also noted in the main text that the magnetic energy spectrum derived from the experimental proton radiography data using (S34) is suppressed at small wavelengths ( $\lesssim 100$   $\mu\text{m}$ ). We emphasize that this may not be indicative of the true spectrum, which could follow a flatter power law – yet this would not be reproduced using the reconstruction method. In essence, this is because the injectivity assumption required above for the reconstruction to be valid is scale-dependent. Small-scale magnetic structures are more likely to lead to the crossing of trajectories of neighboring protons than larger structures of the same field strength, even though the deflections associated with the small structures are smaller. For multi-scale stochastic magnetic fields, this means that the reconstruction algorithm applied to small-scale flux structures will produce an underestimate of small-scale path-integrated fields – which in turns leads to the suppression of small wavelengths in the magnetic energy spectrum. In the limit of very small structures, this lack of injectivity manifests itself diffusively, effectively leading to an additional smearing effect. This phenomenon is demonstrated below for the stochastic magnetic fields produced in the FLASH simulation.

## The collisional approximation

Starting with the measured values for flow velocities, temperatures, magnetic fields, and densities as given by various experimental diagnostics, we can fully characterize the plasma state. The calculated Debye length is  $\lambda_D \approx 7.4 \times 10^{-7}$  cm, which is larger than the ion separation length  $n_i^{-1/3} \approx 3 \times 10^{-7}$  cm: this indicates that the average number of particles in the Debye sphere is large, and hence the plasma can be described classically. The Coulomb logarithm is found to be  $\log \Lambda \approx 7$ .

Assuming an underlying Maxwellian distribution, the ion-ion mean free path is  $\lambda_{ii} \approx 2 \mu\text{m}$ , which (as would be expected for a classical plasma) is larger than the Debye length, but smaller than all relevant hydrodynamic length scales. This would seem to imply that the plasma is collisional. However, we also need to account for the fact that the plasma formation of the central interaction region is due to two counter-propagating streams. The initial distribution function in the interaction region is certainly not Maxwellian. This initial distribution (approximately consisting of a double Maxwellian distribution with peaks centered at  $u = -U$  and  $u = U$ , where  $U \approx 200 \text{ km/s}$ , respectively) will, however, be subject to a variety of processes, including kinetic instabilities and collisions between counter-propagating particles. To estimate the dominant relaxation process, we first note that since, in each jet,

$$\frac{m_i U^2}{2k_B T_e} > 1, \quad (\text{S36})$$

the ion motions are energetically dominant over electron motions. This is equivalent to jet motion having Mach number  $> 1$  before the collision. Therefore, we can approximate (to an order of magnitude) the collisional relaxation times using those of a test ion beam moving with velocity  $2U$  into a Maxwellian plasma at rest [46]. This test beam is fast relative to the ions in the rest frame, but slow compared to the electrons:

$$V_{ti} = 90 \text{ km/s} < U < V_{te} = 9,000 \text{ km/s}, \quad (\text{S37})$$

where  $V_{ti}$  and  $V_{te}$  are the ion and electron thermal speeds, respectively. Estimating the beam relaxation times accordingly, we find that predominant slowing and perpendicular spreading of the test-beam distribution is due to ions. The associated length scales over which particles in the jet experience these relaxation processes are  $\lambda_s \approx 0.015 \text{ cm}$  and  $\lambda_\perp \approx 0.0037 \text{ cm}$ , respectively.

The characteristic scale for the Weibel instability in the jet is [47, 48]  $\ell_{EM} \sim c/\omega_{pi}$ , where  $\omega_{pi}$  is the ion-plasma frequency. For our experimental conditions, we have  $\ell_{EM} \approx 31 \text{ nm}$ . The length scale for the development of electrostatic instabilities is [47]  $\ell_{ES} \approx 0.015 \text{ cm}$ , which is similar in order magnitude to the length scales associated with collisions. This suggests that a number of relaxation processes could be acting initially. However, the Thomson scattering data for a single jet (as discussed above) indicates that the front of the jet has a lower electron (and ion) temperature: this would increase length scales associated with kinetic instabilities, whilst decreasing those of collisions. Furthermore, as the interaction between the jets develops, regions of higher density and lower velocity might be expected, both of which would also favour collisions as the dominant process. Thus, we conclude that it is reasonable to describe the developed interaction-region plasma as approximately Maxwellian, even if the relaxation processes governing the initial jet interaction are not simply collisional. Under this assumption, the temperature equilibration time between ions and electrons is calculated to be  $\tau_{ie}^e \approx 8 \text{ ns}$ , which is consistent with the assumption of a plasma in thermal equilibrium.

Following on from this conclusion, we can estimate various transport coefficients. The appropriate form of these depends on the magnetization of the component species in the plasma;

the Larmor frequencies for electrons and ions (assuming  $B \approx 120$  kG) multiplied by their respective collision times are

$$\Omega_i \tau_{ii} \approx 0.01 \ll 1 \quad \Omega_e \tau_{ie} \approx 2.8 > 1. \quad (\text{S38})$$

This implies that the electrons are weakly magnetized, and ions are entirely unmagnetized. The magnetized state of the electrons has various consequences: anisotropization of the thermal and electrical conductivities and the appearance of various terms in the generalized Ohm's law associated with a finite electron Larmor radius. However, since ion flows dominate bulk motion, it might be inferred that the plasma dynamics would be relatively unaffected by this.

Thus, we conclude that conventional MHD provides a reasonable description of the plasma dynamics. Since  $T_e \sim T_i$ , the electrical conductivity is essentially determined by the electrons, and the viscosity by ions [50]. This gives diffusivities

$$\nu \approx 1,110 \text{ cm}^2/\text{s}, \quad \mu \approx 830 \text{ cm}^2/\text{s}. \quad (\text{S39})$$

A summary of relevant parameters related to the experiment is given in Table 1.

## FLASH 3D simulations

The experimental platform was designed using FLASH radiation-MHD simulations. FLASH is a parallel, multi-physics, adaptive-mesh-refinement (AMR), finite-volume Eulerian code [51, 52]. The code scales well to over a 100,000 processors, and uses a variety of parallelization techniques including domain decomposition, mesh replication, and threading to utilize hardware resources optimally. The code is publicly available\* and allows one to model problems in a wide range of disciplines including astrophysics, cosmology, combustion, fluid dynamics, turbulence, and high-energy-density laboratory plasmas (HEDLP).

To design the experiments, we performed an extensive series of moderate-fidelity 2D cylindrical FLASH radiation-MHD simulations on the Beagle 2 cluster at the University of Chicago followed by a smaller set of high-fidelity 3D FLASH radiation-MHD simulations on the Mira supercomputer at ANL. This simulation campaign is described in detail in a companion paper [24]. The numerical modeling of the experimental platform employed the entire suite of HEDLP capabilities [23, 24] of the FLASH code: three-temperature (3T) MHD solvers [53], non-ideal MHD effects such as magnetic resistivity [23] and Biermann battery [54, 55], heat exchange between ions and electrons, implicit<sup>†</sup> thermal conduction and radiation transport in the multi-group diffusion approximation, 3T tabulated equations of state and material opacities, and laser beams that are modeled with geometric-optics ray-tracing and deposit energy via inverse Bremsstrahlung.

We have used the FLASH code to simulate the experiment and reproduce the diagnostics results as shown in Figure 4 of the main paper. This is illustrated in Figure 11. The computational

---

\*<http://flash.uchicago.edu>

<sup>†</sup>using the HYPRE library, [https://computation-rnd.llnl.gov/linear\\_solvers/software.php](https://computation-rnd.llnl.gov/linear_solvers/software.php)

| Quantity                                                 | Formula                                                                          | Value                                   |
|----------------------------------------------------------|----------------------------------------------------------------------------------|-----------------------------------------|
| Average atomic weight ( $M$ )                            |                                                                                  | 6.5 a.m.u.                              |
| Average ion charge ( $Z$ )                               |                                                                                  | 3.5                                     |
| Temperature after collision ( $T_e = T_i$ )              |                                                                                  | $\sim 450$ eV                           |
| Electron density ( $n_e$ )                               |                                                                                  | $10^{20} \text{ cm}^{-3}$               |
| Outer scale ( $L$ )                                      |                                                                                  | 0.06 cm                                 |
| Turbulent velocity ( $u_L$ )                             |                                                                                  | 100 km/s                                |
| Magnetic field ( $B$ )                                   |                                                                                  | 120 kG                                  |
| Coulomb logarithm ( $\log \Lambda$ )                     | $23.5 - \log n_e^{1/2} T_e^{-5/4} - \sqrt{10 - 5 + \frac{(\log T_e - 2)^2}{16}}$ | $\sim 7$                                |
| Debye Length ( $\lambda_D$ )                             | $7.43 \times 10^2 \frac{T^{1/2}}{(n_e(1+Z))^{1/2}}$                              | $7.4 \times 10^{-7} \text{ cm}$         |
| Sound speed ( $c_s$ )                                    | $9.80 \times 10^5 \frac{[ZT_e + (5/3)T_i]^{1/2}}{M^{1/2}}$                       | $2 \times 10^7 \text{ cm/s}$            |
| Mach number                                              | $u_L/c_s$                                                                        | $\lesssim 1$                            |
| Plasma $\beta$                                           | $4.0 \times 10^{-11} \frac{n_e T}{B^2}$                                          | 125                                     |
| Ion-ion mean free path ( $\lambda_{ii}$ )                | $2.88 \times 10^{13} \frac{T_i^2}{Z^4 n_i \log \Lambda}$                         | $1.9 \times 10^{-4} \text{ cm}$         |
| Electron-ion equilibration time ( $\tau_{ie}^\epsilon$ ) | $3.2 \times 10^8 \frac{MT_e^{3/2}}{Z n_e \log \Lambda}$                          | $8.0 \times 10^{-9} \text{ s}$          |
| Electron Larmor radius ( $\rho_e$ )                      | $3.37 \frac{T_e^{1/2}}{B}$                                                       | $6.0 \times 10^{-4} \text{ cm}$         |
| Ion Larmor radius ( $\rho_i$ )                           | $1.44 \times 10^2 \frac{M^{1/2} T_i^{1/2}}{Z B}$                                 | $1. \times 10^{-2} \text{ cm}$          |
| Viscosity ( $\nu$ )                                      | $1.92 \times 10^{19} \frac{T_i^{5/2}}{M^{1/2} Z^4 n_i \log \Lambda}$             | $1.1 \times 10^3 \text{ cm}^2/\text{s}$ |
| Fluid Reynolds number (Re)                               | $u_L L / \nu$                                                                    | $\sim 600$                              |
| Viscous dissipation scale ( $l_\nu$ )                    | $L / \text{Re}^{3/4}$                                                            | $5.2 \times 10^{-4} \text{ cm}$         |
| Resistivity ( $\mu$ )                                    | $3.2 \times 10^5 \frac{Z \log \Lambda}{T_e^{3/2}}$                               | $8.3 \times 10^2 \text{ cm}^2/\text{s}$ |
| Magnetic Reynolds number (Rm)                            | $u_L L / \mu$                                                                    | $\sim 700$                              |
| Magnetic Prandtl number (Pm)                             | $\text{Rm} / \text{Re}$                                                          | $\lesssim 1$                            |
| Resistive dissipation scale ( $l_\mu$ )                  | $l_\nu / \text{Pm}^{1/2}$                                                        | $4.3 \times 10^{-4} \text{ cm}$         |

Table 1: Summary of relevant plasma parameters related to the experiment. The units system used for all physical quantities in the above formulae is Gaussian CGS, except temperature expressed in eV.

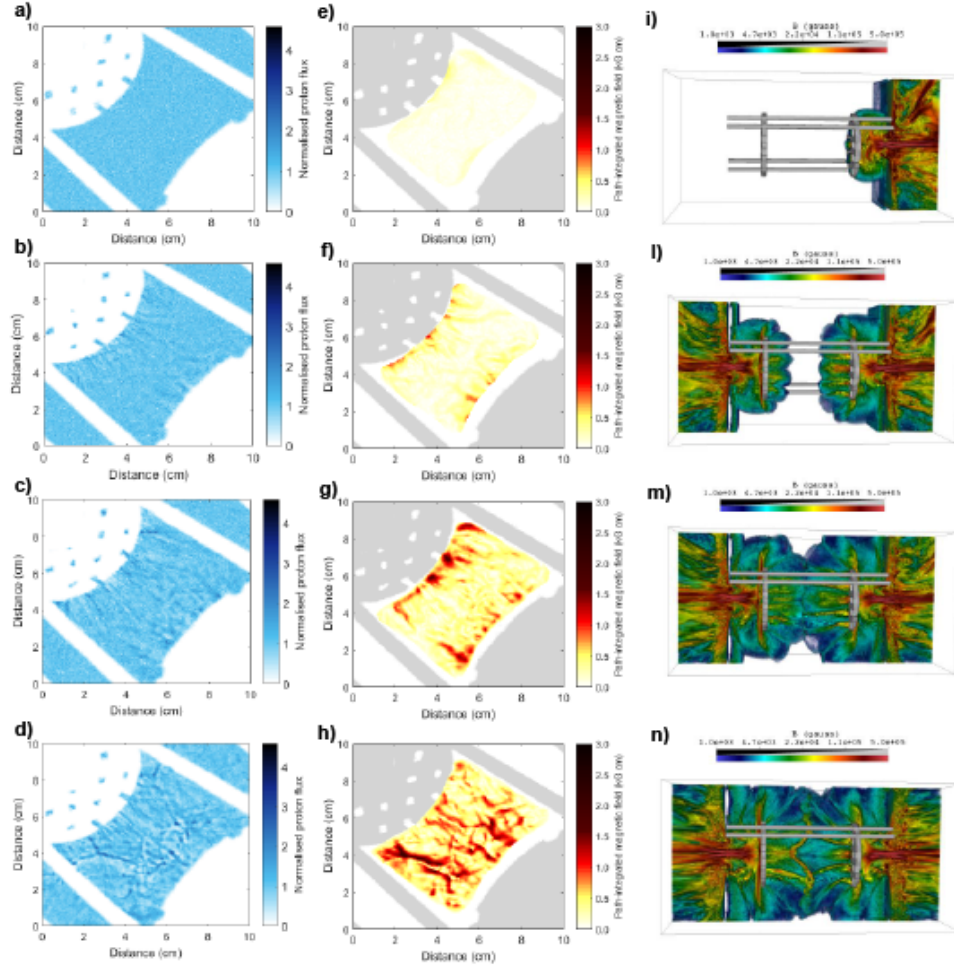

Figure 11: **FLASH simulation results.** Simulated proton radiographs (left column) created by passing a proton beam through FLASH-predicted magnetic fields (right column); path-integrated fields reconstructed from the simulated radiographs (middle column). (a) Simulated number of 15 MeV protons detected on a CR-39 plate. The  $D^3He$  capsule was imploded at  $t = 22$  ns. Fusion reactions occur 0.6 ns after the start of the implosion and the protons are emitted isotropically within a short burst, of  $\sim 150$  ps duration. The flight time of the protons to the plasma is 0.1 ns. This particular target had only grid A and a single plasma flow. The chlorinated plastic foil was driven with a 10 ns long pulse shape (see Figure 1). (b) Same as (a) but with the capsule imploded at  $t = 29$  ns. This target had both our grids and the two chlorinated plastic foils were driven with a 10 ns laser pulse. (c) Same (b), but with the  $D^3He$  capsule imploded at  $t = 34$  ns. (d) Same as (c), but with the chlorinated plastic foils driven with a 5 ns long pulse, which gives higher flow velocities, hence higher magnetic Reynolds numbers and more pronounced structures. (e) Reconstructed path-integrated magnetic fields for case (a). (f) Same for case (b). (g) Same for case (c). (h) Same for case (d). (i) Magnetic field rendering for case (a). (l) Same for case (b). (m) Same for case (c). (n) Same for case (d).

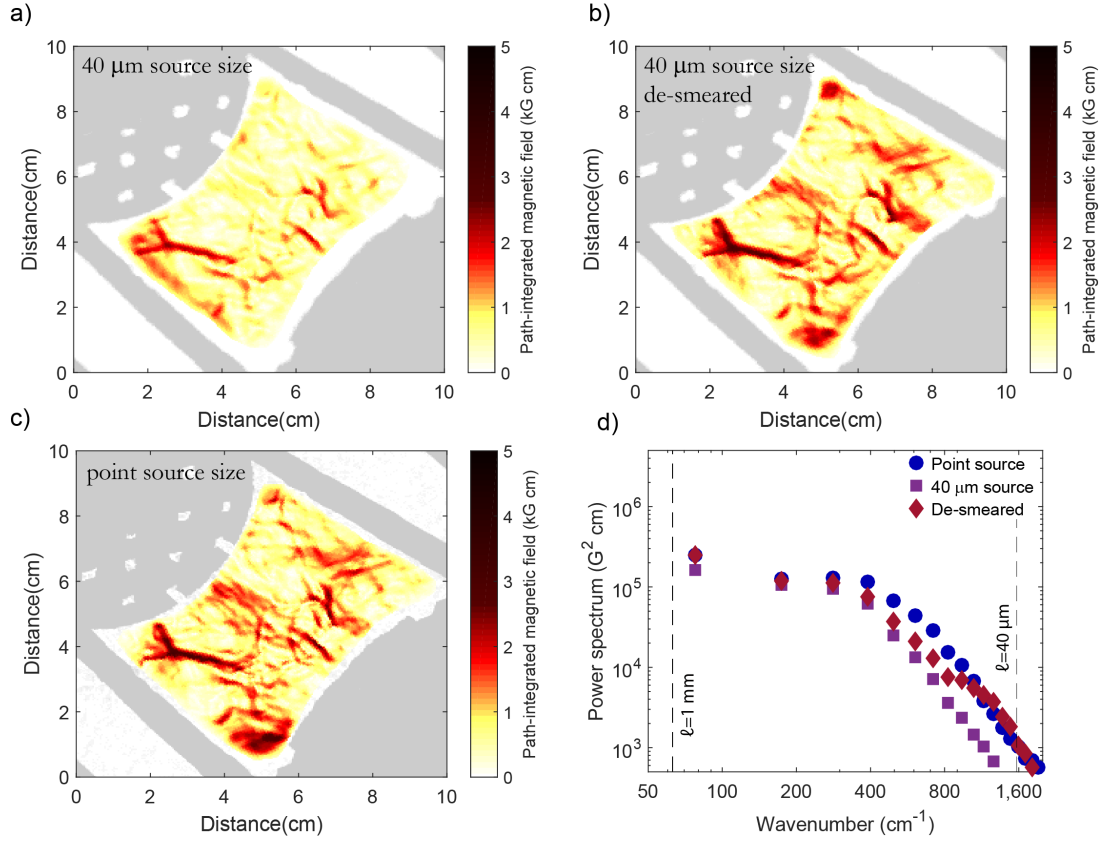

Figure 12: **Effect of proton capsule size.** (a) Synthetic reconstruction of the path-integrated magnetic field from simulated proton radiography images created using a finite-size proton source of diameter  $40\ \mu\text{m}$ . (b) Same as (a) but with the Lucy-Richardson deconvolution scheme included in the reconstruction algorithm. (c) Same as (a) but with a point source of  $2 \times 10^{-6}\ \mu\text{m}$  diameter. (d) Extracted magnetic-field spectra for the three previous cases.

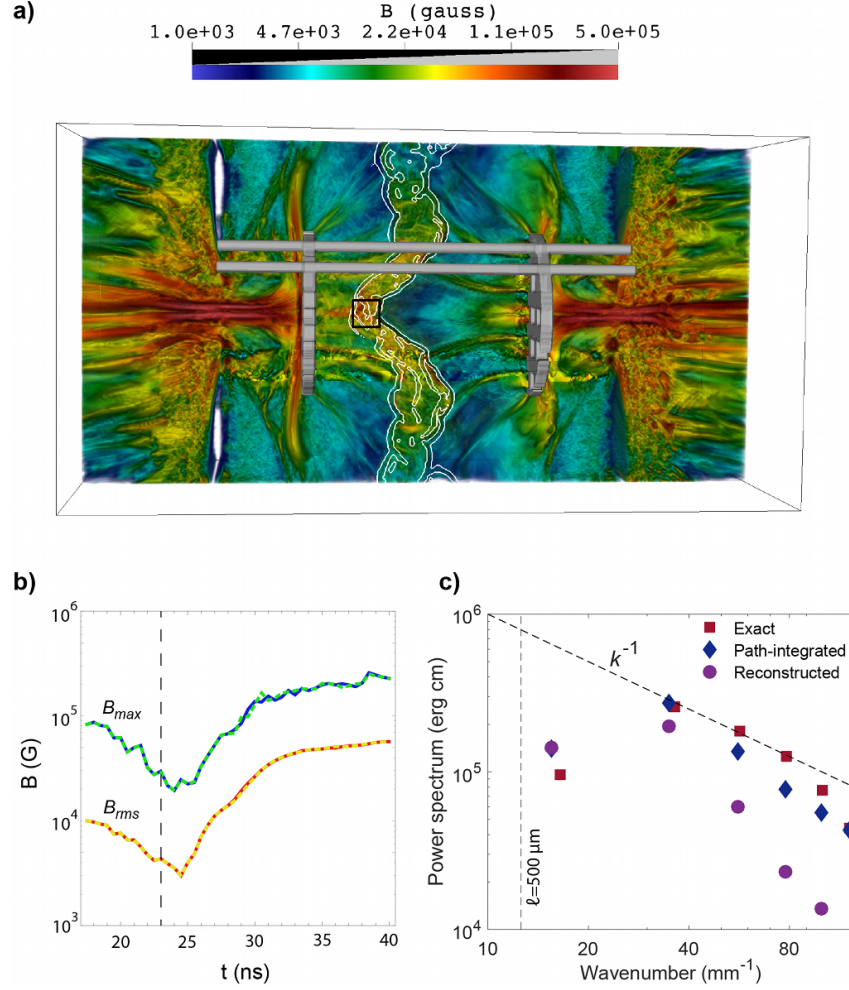

Figure 13: **Magnetic field generation in the jet interaction region.** (a) Rendering of the FLASH magnetic field strength at  $t = 40$  ns for the 5 ns laser drive. The region where the Biermann battery is turned off is outlined by white boundaries. (b) Evolution of maximum field strength,  $B_{max}$ , and the RMS field,  $B_{rms}$ , in the control volume indicated by a square box in panel (a). The plot includes both the results of the full simulation (solid lines), and a simulation where the Biermann battery term was switched off after 23 ns (dashed lines). (c) Magnetic energy spectrum calculated inside the  $500 \mu\text{m}$  control volume using three methods: using FLASH magnetic field values (red squares, see also Figure 2d); integrating the simulated magnetic field in the control volume along the proton probe path (blue diamonds); and from the reconstructed field from FLASH synthetic proton radiography images (purple circles).

domain spans 0.625 cm in the  $X$  and  $Y$  directions, and 1.25 cm along  $Z$  – the line of centers between the two targets. The spatial resolution is  $\sim 25 \mu\text{m}$ . Figure 11 clearly shows the same trend that is seen in the experimental data: a significant increase of the magnetic field following the collision of the two plasma flows. This is reflected in both the change in morphology of the proton radiographs, and in the path-integrated magnetic fields.

The FLASH code can also be used to investigate the efficacy of some of the techniques employed for analyzing the proton radiographs: in particular, the Lucy-Richardson deconvolution scheme used to correct for a finite proton source size, and the calculation of  $B_{rms}$ . Synthetic proton radiographs can be generated using the FLASH simulation with both a point source and a more realistic finite  $40 \mu\text{m}$  source. This allows the reconstructed path-integrated field from the point source to be compared with the reconstructed field from the finite source, both with and without the use of the deconvolution algorithm (Figure 12). Figure 12a shows that without the deconvolution algorithm, the reconstruction process leads to lower field strengths. However, Figure 12b shows that with the deconvolution algorithm, a much closer match is achieved. This is also reflected in the magnetic-field spectra predicted from the proton radiography using (S34). Applying the formula (S35) to predict  $B_{rms}$  for the FLASH simulation in the same region as marked on Figure 4f, but applied to Figure 12b, we obtain  $B_{rms} \approx 55 \text{ kG}$ . In the FLASH simulation, this value can also be calculated directly from the magnetic field: we find that  $B_{rms} = 57 \text{ kG}$ . The predicted and actual values are in reasonable agreement.

As mentioned in the main text, FLASH also gives the magnitude of the RMS field generated initially by the laser interaction as  $\lesssim 4 \text{ kG}$ . We notice, however, that after the collision, the growth of this initial field is only due to the stretching and twisting of the field lines and not any more to the Biermann battery. As shown in Figure 13, FLASH calculations performed with the Biermann battery term turned off for times  $t > 23 \text{ ns}$  do not show any difference with those done including the Biermann effect at all times. This applies to both peak and RMS values of the magnetic field in the interaction region.

The FLASH magnetic fields can also be used to illustrate the phenomenon described above of suppression of small-wavelength structures when reconstructing magnetic spectra from proton radiographs. Figure 13c shows the magnetic energy spectrum derived from the path-integrated field as measured by test protons used for imaging, as well as from the reconstructed path-integrated magnetic field from synthetic proton images of FLASH magnetic fields. The latter in particular shows a much steeper tail than the true FLASH spectrum, with a slope that matches the experimental results of Figure 4g in the main text.

## References and Notes

- [31] P. Arévalo *et al.*, *A Mexican hat with holes: calculating low-resolution power spectra from data with gaps*, Mon. Not. R. Astron. Soc. **426**, 1793 (2012).
- [32] E. Churazov *et al.*, *X-ray surface brightness and gas density fluctuations in the Coma cluster*, Mon. Not. R. Astron. Soc. **421**, 1123 (2012).

- [33] J.E. Cross, B. Reville, and G. Gregori, *Scaling of magneto-quantum-radiative hydrodynamic equations: from laser-produced plasmas to astrophysics*, *Astrophys. J.* **795**, 59 (2014).
- [34] T.A. Ensslin, and C. Vogt, *The magnetic spectrum in Faraday rotation screens*, *Astron. Astrophys.* **401**, 835 (2003).
- [35] J. Cho, and D. Ryu, *Characteristic lengths of magnetic field in magnetohydrodynamic turbulence*, *Astrophys. J* **705**, L90 (2004).
- [36] E.E. Segre, *A review of plasma polarimetry – theory and methods*, *Plasma Phys. Control. Fusion* **41**, R57 (1999).
- [37] A.F.A. Bott, C. Graziani, P. Tzeferacos, D.Q. Lamb, G. Gregori, and A.A. Schekochihin *Proton radiography of small-scale stochastic magnetic fields*, In prep. (2017)
- [38] W. Gangbo, and R.J. McCann, *The geometry of optimal transportation*, *Acta Math.* **177**, 113 (1996)
- [39] M.M. Sulman, J.F. Williams, and R.D. Russell *An efficient approach for the numerical solution of the Monge-Ampere equation*, *Appl. Numer. Math.* **61**, 298 (2011)
- [40] W.H. Richardson, *Bayesian-based iterative method of image restoration*, *JOSA.* **62**, 55 (1972)
- [41] L.B. Lucy, *An iterative technique for the rectification of observed distributions*, *Astron. J.* **79**, 745 (1974)
- [42] F.H. Seguin et. al., *D3He-proton emission imaging for inertial-confinement-fusion experiments*, *Rev. Sci. Instrum.* **75**, 3520 (2004)
- [43] C. Li et. al., *Measuring E and B fields in laser-produced plasmas with monoenergetic proton radiography*, *Phys. Rev. Lett.* **97**, 135003 (2006)
- [44] M. J.-E. Manuel et. al., *Source characterisation and modelling development for monoenergetic-proton radiography experiments on OMEGA*, *Rev. Sci. Instrum.* **83**, 063506 (2012)
- [45] N.L. Kugland et al., *Self-organized electromagnetic field structures in laser-produced counter-streaming plasmas*, *Nat. Phys.* **8**, 809 (2012).
- [46] B.A. Trubnikov, *Particle interactions in a fully ionised plasma*, *Rev. Plasma Phys.* **1** (1965)
- [47] H.-S. Park et al., *Studying astrophysical collisionless shocks with counterstreaming plasmas from high power lasers*, *High Energy Dens. Phys.* **8**, 38 (2012).

- [48] R.P. Drake and G. Gregori, *Design considerations for unmagnetized collisionless-shock measurements in homologous flows*, *Astrophys. J.* **749**, 171 (2012).
- [49] T.N. Kato and H. Takabe, *Electrostatic and electromagnetic instabilities associated with electrostatic shocks: two-dimensional particle-in-cell simulation*, *Astrophys. J.* **681**, L93 (2008).
- [50] S.I. Braginskii, *Transport processes in a plasma*, *Rev. Plasma Phys.* **1**, 205 (1965).
- [51] B. Fryxell *et al.*, *FLASH: an adaptive mesh hydrodynamics code for modeling astrophysical thermonuclear flashes*, *Astrophys. J.* **131**, S273 (2000).
- [52] A. Dubey *et al.*, *Electrostatic and electromagnetic instabilities associated with electrostatic shocks: two-dimensional particle-in-cell simulation*, *Parall. Comp.* **35**, 512 (2009).
- [53] D. Lee, *A solution accurate, efficient and stable unsplit staggered mesh scheme for three dimensional magnetohydrodynamics*, *J. Comp. Phys.* **243**, 269 (2013).
- [54] M. Fatenejad *et al.*, *Modeling HEDLA magnetic field generation experiments on laser facilities*, *High Energy Dens. Phys.* **9**, 172 (2013).
- [55] C. Graziani *et al.*, *The Biermann catastrophe in numerical magnetohydrodynamics*, *Astrophys. J.* **802**, 43 (2015).
